# Supplementary material for: GS-Marker: Generalizable and Robust Watermarking for 3D Gaussian Splatting
Source: arXiv:2503.18718 source file (2025-03-24)
Supplement: Supplementary file 1 [file X_suppl.tex]

\clearpage
\setcounter{page}{1}
\maketitlesupplementary

% \section{Rationale}
% \label{sec:rationale}
% % 
% Having the supplementary compiled together with the main paper means that:
% % 
% \begin{itemize}
% \item The supplementary can back-reference sections of the main paper, for example, we can refer to \cref{sec:intro};
% \item The main paper can forward reference sub-sections within the supplementary explicitly (e.g. referring to a particular experiment); 
% \item When submitted to arXiv, the supplementary will already included at the end of the paper.
% \end{itemize}
% % 
% To split the supplementary pages from the main paper, you can use \href{https://support.apple.com/en-ca/guide/preview/prvw11793/mac#:~:text=Delete%20a%20page%20from%20a,or%20choose%20Edit%20%3E%20Delete).}{Preview (on macOS)}, \href{https://www.adobe.com/acrobat/how-to/delete-pages-from-pdf.html#:~:text=Choose%20%E2%80%9CTools%E2%80%9D%20%3E%20%E2%80%9COrganize,or%20pages%20from%20the%20file.}{Adobe Acrobat} (on all OSs), as well as \href{https://superuser.com/questions/517986/is-it-possible-to-delete-some-pages-of-a-pdf-document}{command line tools}.

\section*{A. Results on Blender Dataset}
\label{sec:blender}
We compare our method with the SOTA 3D watermarking method WateRF on the widely applied Blender dataset \cite{nerf}. For our method, we reconstruct the 3DGS models on the Blender dataset with the official codebase\footnote{https://github.com/graphdeco-inria/gaussian-splatting}, and then generate the watermarked 3DGS by applying our model on the reconstructed 3DGS. Note that we directly use our model trained on the 3DGS dataset built on the Objaverse dataset without re-training or fine-tuning. For WateRF, we train the NeRF models on the Blender dataset using the TensoRF \cite{tensorf} method, followed by applying WateRF on the generated NeRF models to obtain watermarked NeRF. We compute the bit accuracy, PSNR, SSIM, and LPIPS on the test dataset of the Blender dataset, following the conventional literature in NeRF research. The results are demonstrated in \cref{tab.blender}. As shown in this table, our method achieves comparable bit accuracy and better visual quality than WateRF. Moreover, we calculate the average embedding time of both our method and the WateRF on the Blender dataset with an NVIDIA A100 Tensor Core GPU. The results in \cref{tab.blender} show that our method requires much less embedding time than WateRF, which illustrates the superiority of our method. 
\begin{table}
    \begin{center}
    \setlength{\tabcolsep}{2.5pt}
    \resizebox{\linewidth}{!}{
    \begin{tabular}{cccccc}
    % \begin{tabularx}{\textwidth}{XXXXX}
    % \begin{tabular}{p{2.2cm}p{1.3cm}p{1.1cm}p{1.1cm}p{1.1cm}}
    \toprule[1pt]
     & Emb Time & Acc $\uparrow$ & PSNR $\uparrow$ & SSIM $\uparrow$ & LPIPS $\downarrow$ \\
    \hline
    WateRF & 4952 & 93.26 & 30.81 & 0.9472 & 0.0577 \\
    \hline
    % \makecell{CopyRNeRF + 3DGS} & 43.75 & 38.48 & 0.9865 & 0.0289 \\
    % \hline
    Ours & 0.3306 & 93.56 & 33.40 & 0.9828 & 0.0154 \\
    \toprule[1pt]
    \end{tabular}
    }
    \end{center}
    % \vspace{-6pt}
    \caption{The watermark embedding time (s), bit accuracy ($\%$), and visual qualities of our method compared with WateRF on the Blender dataset.}
    % \ca{identify generalizable or not. cite}
% \vspace{-8pt}
\label{tab.blender}
\end{table}

\section*{B. View Variance}
To analyze the robustness of our method and other baseline methods against camera pose variations, we assess the standard deviation of bit accuracy across multiple views of the same object. For each object in our test dataset, we randomly sample 40 camera poses and calculate the bit accuracy for each pose. Subsequently, we compute the standard deviation of these bit accuracy for each object and averaged these values across the dataset. The experimental results is demonstrated in \cref{tab.bit_std}, which indicate that our method achieves a lower standard deviation. The experimental results underscore the enhanced robustness of our method to variations in camera poses.

% which indicate that the standard deviation of bit accuracy for our method and WateRF are $4.00\%$ and $7.17\%$, respectively. While the average bit accuracy of our method and WateRF are $96.07\%$ and $85.27\%$. This experimental results underscores the enhanced robustness of our method to variations in camera poses.

\begin{table}
    \begin{center}
    \setlength{\tabcolsep}{2.5pt}
    \begin{tabular}{ccc}
    \toprule[1pt]
     & Bit Acc mean ($\%$)  & Bit Acc std ($\%$)  \\
    \hline
    Ours & 96.07 & 4.00 \\
    \hline
    WateRF & 83.43 & 7.17 \\
    \toprule[1pt]
    \end{tabular}
    \end{center}
    \caption{The mean value and standard deviation of bit accuracy. The experiments are conducted on message length $l_b=16$}
\label{tab.bit_std}
\end{table}

\section*{C. More Quantitative Results}
We show more rendered images of our model and the baseline methods in \cref{fig:result_supp_img1}. As demonstrated in the figure, our method achieves better bit accuracy and visual quality than other baseline methods.
\begin{figure*}
  \centering
   \includegraphics[width=0.99\linewidth]{Figs/result_supp_img1.pdf}
   \vspace{-8pt}
   \caption{Qualitative comparisons between our method and the baseline. We show the differences (×10) between the images rendered by the input and watermarked 3DGS. Our method achieves better PSNR and bit accuracy than baseline.}
  \label{fig:result_supp_img1}
\end{figure*}
\vspace{-4pt}
